# Supplementary material for: A Bayesian Evaluation Framework for Subjectively Annotated Visual Recognition Tasks
Source: arXiv:2007.06711 source file (2021-09-01)
Supplement: Supplementary file 1 [file auc_table.tex]

\begin{table*}[h]
\begin{center}
\begin{tabular}{|l|llll|llll|llll|llll|}
    \hline
    & \multicolumn{4}{c|}{LabelMe} & \multicolumn{4}{c|}{SCUT-FB5500} & \multicolumn{4}{c|}{APPA-REAL} & \multicolumn{4}{c|}{TestMyBrain: Trust} \\
    & \multicolumn{4}{c|}{Predictor Epochs} & \multicolumn{4}{c|}{Predictor Epochs} & \multicolumn{4}{c|}{Predictor Epochs} & \multicolumn{4}{c|}{Predictor Epochs} \\
    & 0 & 7 & 14 & 100
        & 0 & 3 & 7 & 60
        & 0 & 1 & 2 & 100
        & 0 & 1 & 2 & 100 \\
    \hline
    \textit{Train}: & \multicolumn{4}{c|}{} & \multicolumn{4}{c|}{} & \multicolumn{4}{c|}{} & \multicolumn{4}{c|}{} \\
    AUC
        & .49 & .88 & .99 & .99
        & 0 & 3 & 7 & 60
        & 0 & 3 & 7 & 60
        & 0 & 3 & 7 & 60 \\
    Lower
        & .49 & .88 & .99 & .99
        & 0 & 3 & 7 & 60
        & 0 & 3 & 7 & 60
        & 0 & 3 & 7 & 60 \\
    Upper 
        & .49 & .88 & .99 & .99
        & 0 & 3 & 7 & 60
        & 0 & 3 & 7 & 60
        & 0 & 3 & 7 & 60 \\
    \hline
    \textit{Test}: & \multicolumn{4}{c|}{} & \multicolumn{4}{c|}{} & \multicolumn{4}{c|}{} & \multicolumn{4}{c|}{} \\
    AUC
        & .49 & .87 & .89 & .89
        & 0 & 3 & 7 & 60
        & 0 & 3 & 7 & 60
        & 0 & 3 & 7 & 60 \\
    Lower
        & .49 & .88 & .99 & .99
        & 0 & 3 & 7 & 60
        & 0 & 3 & 7 & 60
        & 0 & 3 & 7 & 60 \\
    Upper
        & .49 & .88 & .99 & .99
        & 0 & 3 & 7 & 60
        & 0 & 3 & 7 & 60
        & 0 & 3 & 7 & 60 \\
    \hline
\end{tabular}
\end{center}
%\vspace{-6mm}
\caption{
    The values of the original AUC and the lower and upper bounds of the BNN's highest density credible interval as visualized in Supp. Mat. Fig \ref{fig:exp3_auc}.
}
\label{tab:auc}
\end{table*}
